# Supplementary material for: A Panda? No, It's a Sloth: Slowdown Attacks on Adaptive Multi-Exit Neural Network Inference
Source: arXiv:2010.02432 source file (2021-02-25)
Supplement: Supplementary file 1 [file advtrain_attacks_100.tex]

% : table...
\begin{table}[ht]
	\centering
	\caption{\textbf{Evaluating adversarially-trained models against slowdown attacks.} Each entry includes the model's efficacy (\emph{left}) and accuracy (\emph{right}). Results are on CIFAR-10, in the RAD$<$5\% setting.}
	\begin{sc}
		\adjustbox{max width=\textwidth}{%
		\begin{tabular}{@{}c c cccc c@{}}
			\toprule
			\textbf{Adv. Training} & \textbf{No Attack} & \textbf{PGD-100} & \textbf{PGD-100 (Avg.)} & \textbf{PGD-100 (Max.)} & \textbf{UAP} & \textbf{Ours} \\ \midrule
			\textbf{Vanilla} & 0.73 / 89\% & 0.82 / 20\% & 0.89 / { }{ }6\% & 0.84 / 16\% & 0.71 / 56\% & 0.00 / 14\% \\
			\textbf{PGD-10} & 0.64 / 89\% & 0.54 / 46\% & 0.77 / 13\% & 0.65 / 20\% & 0.65 / 81\% & 0.34 / 77\% \\
			\textbf{PGD-10 (Avg.)} & 0.64 / 81\% & 0.55 / 46\% & 0.58 / 39\% & 0.59 / 41\% & 0.64 / 81\% & 0.40 / 77\% \\
			\textbf{PGD-10 (Max.)} & 0.64 / 81\% & 0.56 / 44\% & 0.60 / 32\% & 0.59 / 35\% & 0.64 / 81\% & 0.37 / 78\% \\
			\midrule
			\textbf{Ours} &   &   &   &   & - & \textbf{-} \\
			\bottomrule
		\end{tabular}
	}
	\end{sc}
	\label{tbl:sup-advtrain-attacks-100}
\end{table}
